# Supplementary material for: Re-ReND: Real-time Rendering of NeRFs across Devices
Source: arXiv:2303.08717 source file (2023-03-15)
Supplement: Supplementary file 1 [file appendix.tex]

\documentclass[10pt,twocolumn,letterpaper]{article}
\usepackage{multirow}
\usepackage{iccv}
\usepackage{times}
\usepackage{epsfig}
\usepackage{graphicx}
\usepackage{amsmath}
\usepackage{amssymb}

%%%%% Sara added this packages
% \usepackage{multirow}
\usepackage{booktabs}
\usepackage{mathtools}
\usepackage{enumerate}
\usepackage{adjustbox}
\usepackage{comment}
\usepackage{xcolor}
\usepackage{nicefrac}

%%%%% Sara finished 
% Include other packages here, before hyperref.

% If you comment hyperref and then uncomment it, you should delete
% egpaper.aux before re-running latex.  (Or just hit 'q' on the first latex
% run, let it finish, and you should be clear).
\usepackage[breaklinks=true,bookmarks=false]{hyperref}

%%%%% Sara added this packages
\definecolor{DarkGreen}{rgb}{0.0, 0.7, 0.5}

% Support for easy cross-referencing
\usepackage[capitalize]{cleveref}
\crefname{section}{Sec.}{Secs.}
\Crefname{section}{Section}{Sections}
\Crefname{table}{Table}{Tables}
\crefname{table}{Tab.}{Tabs.}

\makeatletter
\DeclareRobustCommand\onedot{\futurelet\@let@token\@onedot}
\def\@onedot{\ifx\@let@token.\else.\null\fi\xspace}

\newcommand{\Table}[1]{Table~\ref{tab:#1}}
\newcommand{\Figure}[1]{Figure~\ref{fig:#1}}

\newcommand{\methodname}{Re\nobreakdash-ReND\xspace}

\usepackage{array}
\newcommand{\thickhline}{%
    \noalign {\ifnum 0=`}\fi \hrule height 1pt
    \futurelet \reserved@a \@xhline
}
\newcolumntype{"}{@{\hskip\tabcolsep\vrule width 1pt\hskip\tabcolsep}}
%%%%% Sara finished

% \iccvfinalcopy % *** Uncomment this line for the final submission

 % *** Enter the ICCV Paper ID here

% Pages are numbered in submission mode, and unnumbered in camera-ready
\ificcvfinal\pagestyle{empty}\fi

\begin{document}

%%%%%%%%% TITLE - PLEASE UPDATE
\title{Re-ReND: Real-time Rendering of NeRFs across Devices \\
\large Appendix \\}  % **** Enter the paper title here

\maketitle
\textcolor{red}{\textbf{[Please read: \textit{erratum}.]}} Table 2 of the main manuscript contains a clerical error, whereby the reported PSNR value for our method in the synthetic dataset is \textbf{29.70}, while it should be \textbf{29.00}. 
We apologize for this mistake.
We would like to emphasize that this error leaves the paper's main contributions unaffected. 
The corrected table is provided in \Table{PSNRsyn}: row corresponding to $18$ texels, column \textit{``aver.''}. 
% We thank the readers for their attention to detail.

Next, we present the Supplementary Materials for the paper ``Re-ReND: Real-time Rendering of NeRFs across Devices''.
Specifically, in addition to the results reported in the paper, we report results of \methodname w.r.t. Image Quality~(Section~\ref{sec:im_qual}) and (Section~\ref{sec:quali}), Rendering Speed~(Section~\ref{sec:fps}), Mesh Size~(Section~\ref{sec:mesh_size} and Section~\ref{sec:meshi}), Disk Space~(Section~\ref{sec:disk_space}), validation of view-dependent effects (Section~\ref{sec:val}),  sensitivity to geometry variations (Section~\ref{sec:geo}) and Photo-metric quality w.r.t. embedding dimensionality $D$ (Section~\ref{sec:dim}).
Furthermore, we encourage the reviewers to watch the \textbf{attached video}, \texttt{Re-ReND.mp4}, demonstrating \methodname's capabilities of real-time rendering across devices.
% In particular, please refer to .
This video demonstrates how \methodname can render, in real time, a scene composed of tens (\Figure{composit}) or even thousands (\Figure{many_objects}) of objects. % , respectively. %  , or even with thousands of . %  in an AR headset.
\Figure{composit} illustrates such a scene, composed of moving chairs, hotdogs, the drumset, and a microphone.

Finally, we also provide the PyTorch~\cite{NEURIPS2019_9015} and GLSL implementations of our method inside the folders called \texttt{Re-ReND\_Pytorch\_code} and \texttt{Re-ReND\_GLSL\_code}.

% \thispagestyle{empty}
% \appendix

%%%%%%%%% BODY TEXT - ENTER YOUR RESPONSE BELOW
% \section{The PyTorch code and GLSL code}

%  \begin{itemize}
%     \item Clean and README.md
%     \item Should I upload only pur method or MipNeRF and NeRF++?
%     \item Should I upload the generated data and the meshes in a google drive? What happens with anonymity?
% \end{itemize}

% \section{A video showing how we were measuring the FPS}
% \section{A video showing real scenes in comparison with MobileNeRF and SNeRG}
% \section{Qualitative Results}

%  \begin{itemize}
%     \item all objects visualizations 
% \end{itemize}

%-------------------------------------------------------------------------

\input{supplmat/sections/quantitative.tex}
%------------------------------------------------------------------------
% \section{Scene editing: compositing (1000 chairs or removing part of the scene, combining backgrounds??)}

%-------------------------------------------------------------------------
% \section{Inflating objects, sphere, convex hull...}

%%%%%%%%% REFERENCES
\clearpage
{\small
\bibliographystyle{ieee_fullname}
\bibliography{egbib}
}

\end{document}
