# Supplementary material for: Re-ReND: Real-time Rendering of NeRFs across Devices
Source: arXiv:2303.08717 source file (2023-03-15)

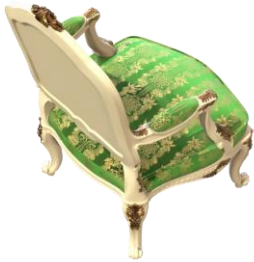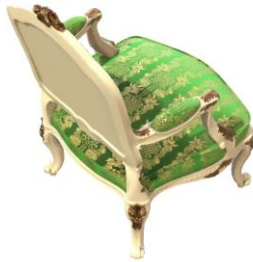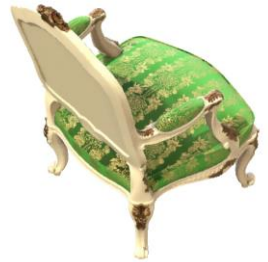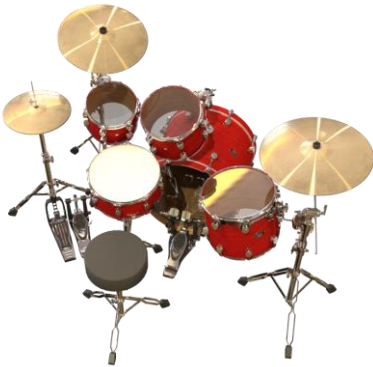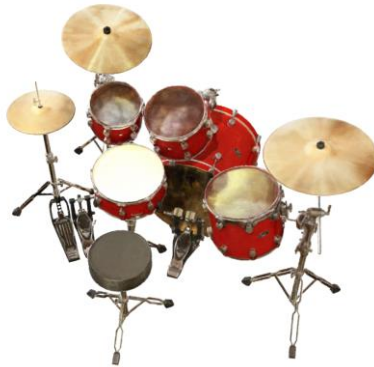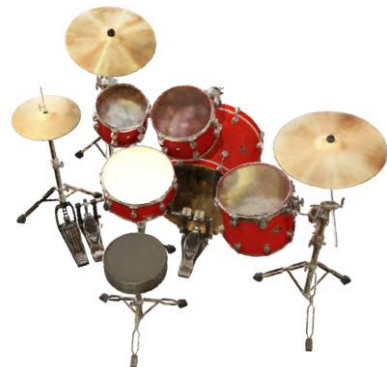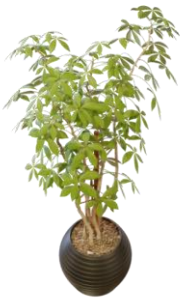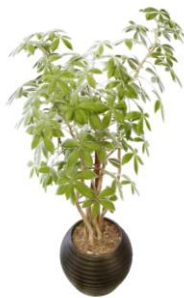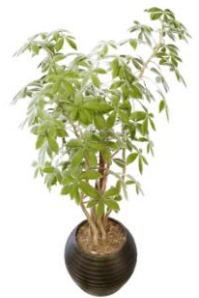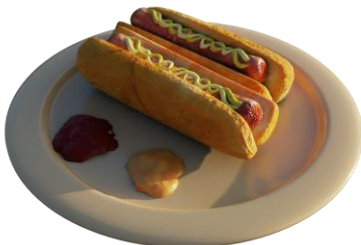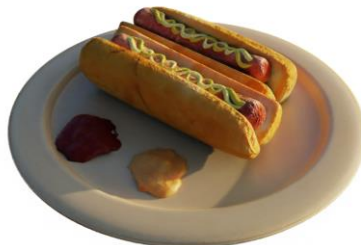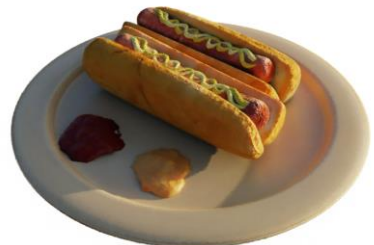

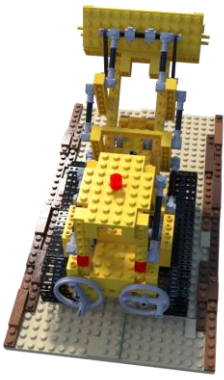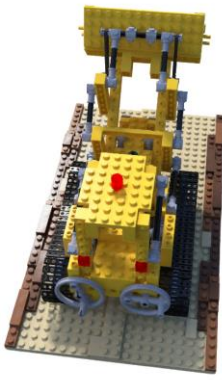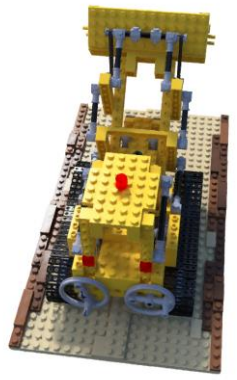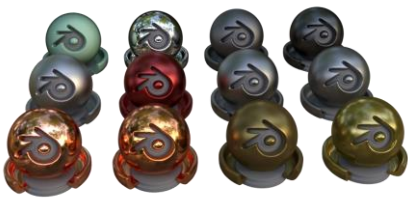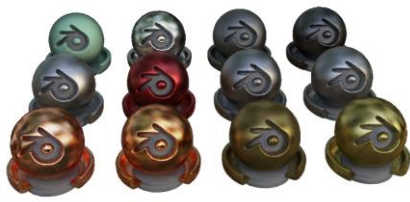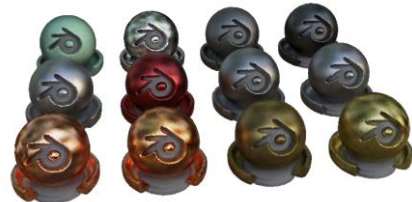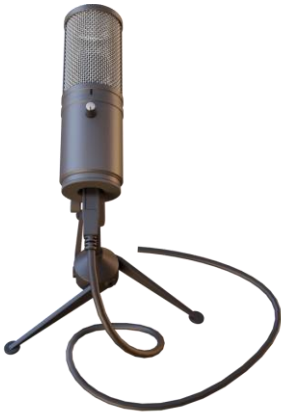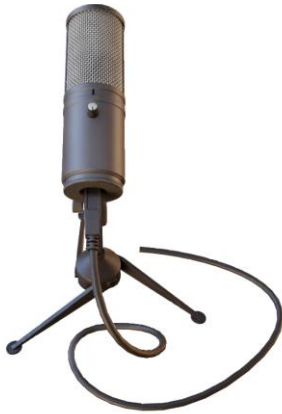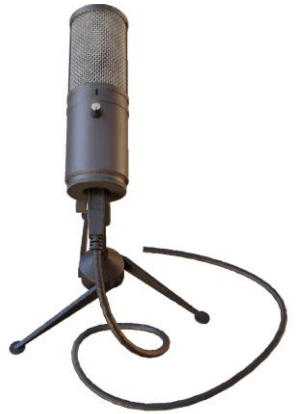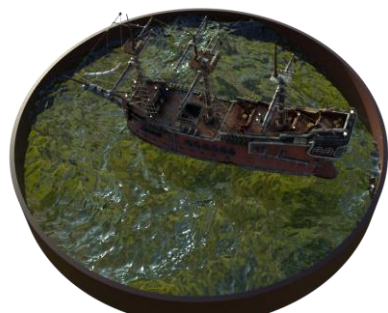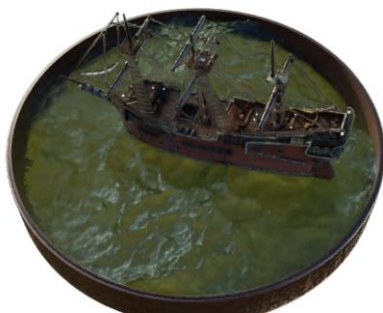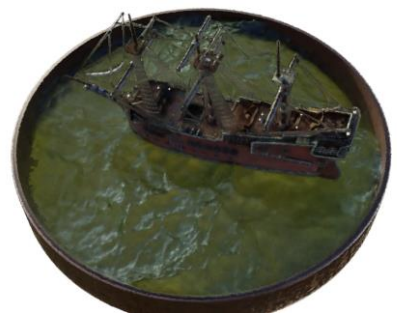

Supplement: Supplementary file 2 [file rerend.pdf]
